# Supplementary material for: High-Dimensional Uncertainty Quantification via Active and Rank-Adaptive Tensor Regression
Source: arXiv:2009.01993 source file (2021-02-02)
Supplement: Supplementary file 1 [file appendix.tex]

%\appendix
\appendices
\section{Basis Function Construction}
\label{sec:TTR}
